# Supplementary material for: Storage and analysis of light-matter entanglement in a fibre-integrated system
Source: arXiv:2201.03361 ancillary file (2022-01-10)
Supplement: Supplementary file 1 [file SM_v4.pdf]

# Supplementary Material for: Storage and analysis of light-matter entanglement in a fibre-integrated system.

Jelena V. Rakonjac,[1*] Giacomo Corrielli,[2*] Dario Lago-Rivera,[1*]
Alessandro Seri,[1] Margherita Mazzera,[3] Samuele Grandi,[1†]
Roberto Osellame[2] and Hugues de Riedmatten[1,4]

[1]ICFO-Institut de Ciencies Fotoniques, The Barcelona Institute of Science and Technology,
08860 Castelldefels (Barcelona), Spain.
[2]Istituto di Fotonica e Nanotecnologie (IFN) - CNR,
P.zza Leonardo da Vinci 32, 20133 Milano, Italy.
[3]Institute of Photonics and Quantum Sciences, SUPA, Heriot-Watt University,
Edinburgh EH14 4AS, UK
[4]ICREA-Institució Catalana de Recerca i Estudis Avançats, 08015 Barcelona, Spain.
† samuele.grandi@icfo.eu
∗ these authors contributed equally

## 1 Waveguide fabrication and fibre-pigtailing

The integrated storage device is based on a type I waveguide femtosecond-laser-written in a $Pr^{3+}$:$Y_2SiO_5$ crystal [1]. It was fabricated by focussing the second harmonic of an Yb-based femtosecond laser source (pulse duration of 300 fs, pulse energy of 40 nJ, repetition rate of 20 kHz, 520 nm wavelength) within the bulk of a $Pr^{3+}$:$Y_2SiO_5$ sample with a dopant concentration of 0.05% (grown by Scientific Materials), and by translating the sample along the $b$ crystallographic axis at the constant speed of 100 $\mu$m/s. The focussing optic used was a 0.65 numerical aperture microscope objective and the focussing depth was 100 $\mu$m below the top surface. The waveguide fabricated in this way supports the propagation of a single mode at 606 nm polarised along the D2 direction, showing a Gaussian mode intensity profile with $e^{-2}$ full widths of 3.1 $\mu$m x 6.0 $\mu$m. The fibre-pigtailing was performed by butt-coupling two 7 m long fibre patch cables (model 630HP) at both the input and the output of the waveguide, and gluing them to the waveguide chip by means of a UV-curing transparent resin (DELO Photobond GB345). Before gluing, each fibre was cleaved and inserted in a 3 mm long glass ferrule with external diameter

of 1 mm. The $e^{-2}$ diameter of the fibre mode intensity profile, measured at 606 nm, is 2.9 $\mu$m. The butt-coupling efficiency is estimated to be 67% per facet by performing the superposition integral between the mode profiles of the fibre and the waveguide, leading to a theoretical maximum transmission efficiency of the overall device of 45%. Waveguide propagation loss, imperfect waveguide facets and fibre splicing required for mounting the device into the cryostat further reduced the overall transmission to 25%. Recent advances in fabrication techniques have allowed us to demonstrate fibre-to-fibre transmissions of 70%, and new waveguide designs could improve the overlap with the fibre mode.

# 2 Entanglement source

To generate narrow photon pairs we insert a type I periodically-poled lithium niobate crystal (PPLN, fabricated by HC Photonics) into an optical cavity. As a consequence, only the photon pairs compatible with the cavity modes will be created. In our case, we pump the PPLN crystal with continuous-wave laser light at 426 nm in order to produce a signal photon at 606 nm and an idler photon at 1436 nm. Thanks to the cavity we obtain a biphoton linewidth of 1.8 MHz, compatible with single-class AFC storage in $Pr^{3+}$ions.

The pump laser is a frequency-doubled laser diode (TOPTICA TA-SHG 110) that generates 426 nm light from a seed at 852 nm through second harmonic generation. A portion of the seed laser is used for Pound-Drever-Hall (PDH) locking to a Fabry-Perot cavity, which ensures that coherence time of the laser is much greater than the coherence time of the biphotons, allowing for the generation of energy-time entangled photons pairs. The source cavity is locked with the PDH technique using a reference beam taken from the memory preparation. In this manner the signal photons are at the same frequency as the AFC.

The spectrum of the emission is actually multimode in frequency [2]. The idler photons are spectrally filtered with a Fabry-Perot cavity (80 MHz of linewidth and 17 GHz of free spectral range), while the signal photons are sent through an etalon filter (4.25 GHz of linewidth and 100 GHz of free spectral range). Moreover, the $Pr^{3+}$:$Y_2SiO_5$ crystal, both with a transparency window or an AFC, acts as a 4 MHz wide band-pass filter. Idler photons are detected with a superconducting nanowire single photon detector (ID281, from ID Quantique, detection efficiency of 80% and 14 Hz of dark counts), while the signal photons are detected with avalanche single photon counters (COUNT-10C-FC and COUNT-20C-FC, from Laser Components; heralded autocorrelation measurements used COUNT-50C-FC). Detection signals are then analysed using a time-to-digital converter (Signadyne).

We study the correlations between the idler and the signal photons through second order cross-correlation measurements where $g^{(2)}_{s,i}= \frac{p_{s,i}}{p_s \cdot p_i}$. Here, $p_{s(i)}$ corresponds to the probability of detecting a signal (idler) photon in a time window $\Delta t$, while $p_{s,i}$ is the probability of detecting a coincidence in that window. We characterise the photon pairs by studying the dependence of $g^{(2)}_{s,i}$ with the pump power sent to the cSPDC. The result is shown in Fig. 1. For this measurement we stored the signal photons for 2 $\mu$s in the AFC.

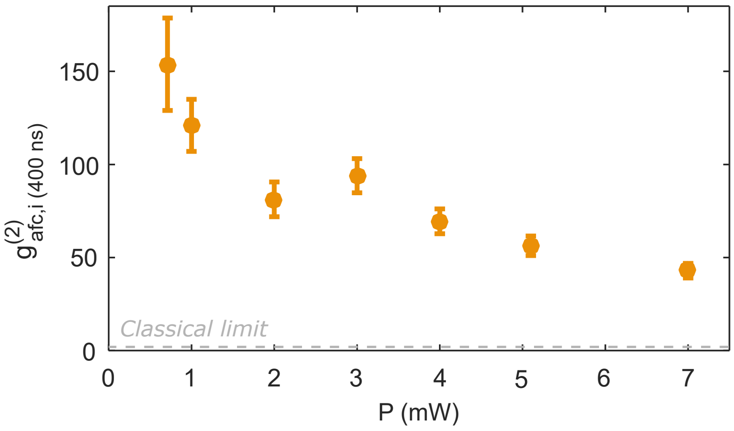


Figure 1: Correlations with varying pump power. $g^{(2)}_{s,i}$ as a function of the pump power of the SPDC source.

# 3 Memory setup

The fibre-pigtailed waveguide is placed inside a closed-cycle cryostat (Optistat AC-V14, Oxford Instruments), that cools the sample to about 2.7 K. We designed a special mount for the cryostat, to hold the crystal and suppress the strong mechanical vibrations on the cold finger of the cryostat, that comes from the cryostat cycle. The mount sits on springs, that decouple the crystal from the vibrations degrading the coherence of the ions, and has a portion of the optical fibre from the fibre pigtails coiled around it, to ensure good thermalisation of the sample and to make sure that the crystal and the pigtails move in unison, therefore avoiding further mechanical stress. This vibration isolation system was only possible because our device is fibre-coupled, as, when coupling to it in free-space, the transmission through the waveguide would vary due to residual oscillations of the sample, induced by the cryostat motion. As mentioned in the main text, the sample maintained the same transmission through several cooling-and-warming cycles. The fibre-to-fibre transmission through the device, from after the source to after the second fibre-pigtail, dropped from 25% to 20% due to the losses of the splicing points and transmission through the 90:10 beam splitter.

We use a frequency-doubled laser diode (TOPTICA TA-SHG Pro) to generate the light at 606 nm for the preparation of the AFC. The seed laser at 1212 nm is locked through PDH technique to a home-built Fabry-Perot cavity that reduces its linewidth to $< 10$ kHz. A portion of the laser is used to address Pr ions in the crystallographic site 1, and is shaped in frequency and time using double-pass acousto-optic modulators controlled by a fast arbitrary waveform generator (Signadyne/Keysight). The final preparation light is coupled to the waveguide through a 90:10 fibre beam splitter that is spliced directly to the pigtail of the waveguide. Signal photons are coupled to the memory using the high transmittivity port of the same beam splitter.

# 4 Analysers

We used unbalanced Mach-Zehnder interferometers to perform full qubit tomography in the time domain. Each consists of two arms made out of optical fibre: one short arm with polarisation control and one long arm with a 90 m fibre spool, and a piezoelectric cylinder with fibre coiled around it. This is used to stretch the optical fibre and stabilise the length difference of the two interferometer arms. The delay introduced by the long arm with respect to the short one is about 420 ns. Besides these common features, the design of the idler interferometer and the signal interferometer differs in the following manner:

- Idler interferometer: It is built with SMF28 optical fibre. In order to stabilise it, we send classical light at 1436 nm that we obtain through a difference frequency generation (DFG) process inside the SPDC source. This DFG light follows the same optical path as the idler photons and it is eventually blocked with a chopper wheel in order to protect the single photon detectors.

- Signal interferometer: It is built with 630HP optical fibre. Laser light at 606 nm is injected into the interferometer through its second output, and is used as a reference signal for its stabilisation. Similarly to the previous case, we use synchronised chopper wheels in order to protect the single photon detectors.

For both interferometers we use the interference of their respective classical references to obtain a locking signal. We select one point in the interference fringe with a side-fringe lock, and the fibre stretcher to maintain the same value of relative phase between the two interferometer arms. We noted that by choosing a locking point in the bottom half of the interference fringe the system was less sensitive to laser power fluctuations.

# 5 Tomography

In this section we describe in detail the two-qubit tomography that we perfomed on the entangled state of the telecom idler photon and the signal, stored as a delocalised excitation in the $Pr^{3+}$:$Y_2SiO_5$ waveguide. We describe the theoretical background, the data acquisition process and the analysis of the results.

## 5.1 Measurement

In order to calibrate the phase settings of each of the interferometers, we performed a quick calibration at the beginning of each tomographic measurement. We locked the phase of the idler interferometer to a value close to the the bottom of its interference fringe to minimise the effect of amplitude oscillations. We then prepared a transparency window in the Praseodymium absorption and measured idler-signal coincidences after the signal interferometer. We studied the variation of these coincidences as a function of the relative phase between the arms of the signal

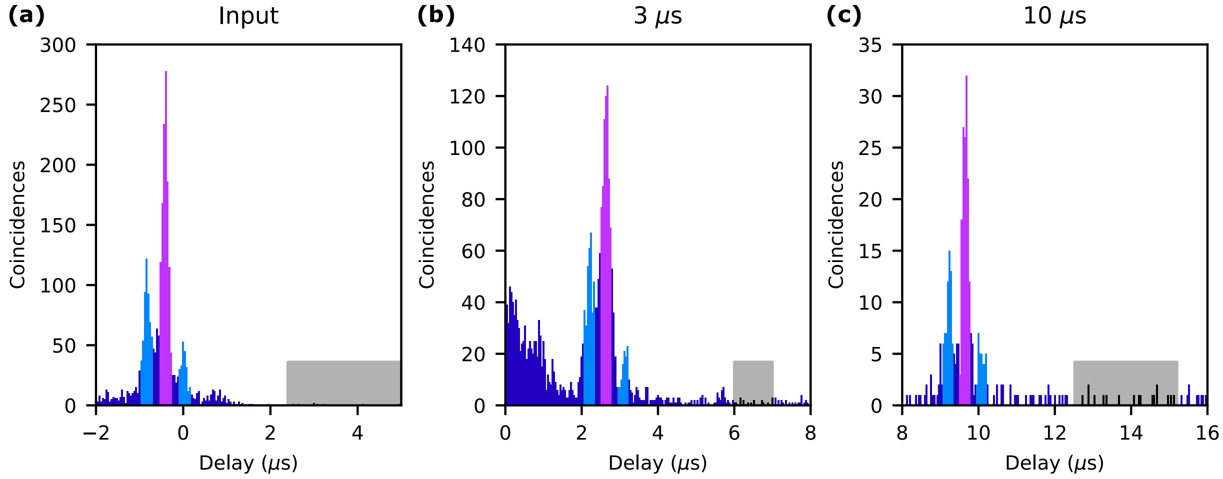


Figure 2: Histograms of signal-idler coincidences for the case of a transparency window, 3 $\mu$s and 10 $\mu$s prepared in the quantum memory. The left, light blue area is the window selected for the projection on $|l\rangle_{\mathrm{s}}$, the right one for $|e\rangle_{\mathrm{s}}$, and the central purple one is the window associated to a superposition of the two. The black shaded area is the region where dark counts were calculated.

interferometer. From this measurement we were able to extract the voltage settings that would yield measurements on the $|\pm\rangle_{\mathrm{s}} = (|e\rangle_{\mathrm{s}} \pm |l\rangle_{\mathrm{s}})/\sqrt{2}$ basis or on the $|R/L\rangle_{\mathrm{s}} = (|e\rangle_{\mathrm{s}} \pm i\,|l\rangle_{\mathrm{s}})/\sqrt{2}$ one. For our cases, these corresponded to locking the signal interferometer to a minimum/-maximum (depending on the interferometer output considered) or to a point shifted by $\pi/2$, respectively. We then acquired signal-idler coincidences, locking the signal interferometer at these two points. The next step was to lock the idler interferometer to a new position, shifted by $-\pi/2$ with respect to the previous one, and repeat the calibration scan of the signal interferometer. With this second fringe we were able to confirm the exact phase shift imparted by the new locking position of the idler interferometer. We again acquired signal-idler coincidences, for the same phase/voltage values of signal interferometer used in the previous acquisition. Finally, we disconnected only the short arm and subsequently only the long arm of the idler interferometer and measured once more with the same voltage locking settings. The same procedure was used for all the three results reported in the main text: transparency windows, 3 $\mu$s and 10 $\mu$s AFC.

Typical idler-signal coincidence histograms are reported in Fig. 2. The central peaks, highlighted in purple, correspond to the measurement on the $|\pm\rangle_{\mathrm{s}}$ basis or on the $|R/L\rangle_{\mathrm{s}}$ one, depending on the setting of the signal interferometer. The two side peaks, in light blue, are the cases of idler and signal photons passing through different arms of the interferometers, and correspond to the measurement of the $|e\rangle_{\mathrm{s}}$ (right peak) and $|l\rangle_{\mathrm{s}}$ (left peak) basis elements. This perhaps counter-intuitive definition of the ealy and late bins is due to the fact that in the histograms the time axis represents the time between the detection of an idler and the detection of a signal. An idler that would pass through the long arm would be delayed, therefore resulting in a shorter interval between its detection and that of its signal counterpart.

## 5.2 Analysis

Since we measured counts at only one of the outputs of the idler interferometer, but on both outputs of the signal interferometer, the measurements described in the previous section corresponds to projections on $|+\rangle_{\mathrm{i}}$, $|L\rangle_{\mathrm{i}}$, $|e\rangle_{\mathrm{i}}$ and $|l\rangle_{\mathrm{i}}$ for the idler and on $|+/-\rangle_{\mathrm{s}}$, $|R/L\rangle_{\mathrm{s}}$ and $|e/l\rangle_{\mathrm{s}}$ for the signal. We could then perform a complete tomography of the entangled state of idler and signal [3], as well as compute 1-qubit tomographies for the states prepared after the detection of an idler. For each experimental setting, we normalised the raw coincidences to the number of idler counts, and calculated $m_j = \frac{N_j}{N_j+N_j'}$, where $N_j$ and $N_j'$ are the normalised coincidences measured for the same $j$-th experimental settings and for two orthogonal basis elements (for projections onto $|+/-\rangle_{\mathrm{s}}$, $|R/L\rangle_{\mathrm{s}}$ these are coincidences at opposite outputs of the signal interferometer). Values of coincidences for projections on $|e\rangle_{\mathrm{s}}$ and $|l\rangle_{\mathrm{s}}$ are summed over all those collected for every signal interferometer setting, and from both outputs of the signal interferometer. We used these values of $m_j$ to run a maximum-likelihood tomography using the Quantum Tomography python package[1]. The different $m_j$ are reported in Table 1, and the results of the tomography are reported in Table 2, where the errors are calculated by simulating 1000 datasets.

Our data analysis up to this point assumes that the measurement settings were correct, i.e. that the phase settings on idler and signal interferometers were accurate. From the phase difference $\phi$ between the short and long arm of the signal or idler interferometer, we can write the projection measurement $M(\phi)$ as:

$$M(\phi) = |\psi\rangle\langle\psi| \text{ with } |\psi\rangle = \frac{|e\rangle + e^{i\phi}\,|l\rangle}{\sqrt{2}}. \tag{1}$$

As mentioned before, we selected two phase settings on the idler interferometer, separated by $\pi/2$ and corresponding to the projections $M_{\mathrm{i}}(0) = |+\rangle\langle+|$ and $M_{\mathrm{i}}(-\pi/2) = |L\rangle\langle L|$. For each of these phases we measured coincidences for two settings of the signal interferometer and in both outputs. These corresponded to the projections $M_{\mathrm{s}}(0) = |+/-\rangle\langle+/-|$ and $M_{\mathrm{s}}(\pi/2) = |R/L\rangle\langle R/L|$. We can recover the exact $M(\phi)$ used for the measurements by analysing the two calibration interference fringes acquired before each tomography run. We ran a least-squares minimisation algorithm that fitted both fringes to two sinusoidals with a common period. In this way, we could relate the phase of each fringe to the voltage values of the signal interferometer used for the measurements, and calculate the exact projective measurements $\widetilde{M}_{\mathrm{s}}(\phi)$ related to the specific signal interferometer setting. At the same time, we could use the difference between the two phases to calculate the exact shift between the two projective measurements on the idler side, and calculate the precise $\widetilde{M}_{\mathrm{i}}(\phi)$. Errors on these phase values were obtained by simulating datasets corresponding to the fringes for 1000 times, using a Poissonian distribution for the measured coincidences, and calculating the phase shifts each time. The tomographies obtained with these corrected projection measurements yielded results close to the previous case, and are those reported in the main text and in the second column of Table 2. In the error

[1] http://www.physics.uiuc.edu/research/QuantumPhotonics/Tomography/

| **INPUT** | | $\hat{M}_s$ | | | | | |
|---|---|---|---|---|---|---|---|
| | | $\|+\rangle\langle+\|$ | $\|-\rangle\langle-\|$ | $\|R\rangle\langle R\|$ | $\|L\rangle\langle L\|$ | $\|l\rangle\langle l\|$ | $\|e\rangle\langle e\|$ |
| $\hat{M}_i = \|+\rangle\langle+\|$ | coinc | 46.09 | 6.18 | 31.45 | 19.71 | 71.42 | 68.01 |
| | DC | 0.04 | 0.07 | 0.04 | 0.04 | 0.18 | 0.18 |
| | idlers | $2.8\cdot10^5$ | $2.8\cdot10^5$ | $2.6\cdot10^5$ | $2.6\cdot10^5$ | $1.1\cdot10^6$ | $1.1\cdot10^6$ |
| $\hat{M}_i = \|L\rangle\langle L\|$ | coinc | 24.08 | 25.78 | 46.92 | 6.79 | 74.09 | 69.31 |
| | DC | 0.08 | 0.12 | 0.04 | 0.08 | 0.322 | 0.322 |
| | idlers | $2.6\cdot10^5$ | $2.6\cdot10^5$ | $2.4\cdot10^5$ | $2.4\cdot10^5$ | $1\cdot10^6$ | $1\cdot10^6$ |
| $\hat{M}_i = \|e\rangle\langle e\|$ | coinc | 13.45 | 14.98 | 15.24 | 11.40 | 13.91 | 115.12 |
| | DC | 0 | 0.10 | 0.12 | 0 | 0.23 | 0.23 |
| | idlers | $9.8\cdot10^4$ | $9.8\cdot10^4$ | $8.1\cdot10^4$ | $8.1\cdot10^4$ | $3.6\cdot10^5$ | $3.6\cdot10^5$ |
| $\hat{M}_i = \|l\rangle\langle l\|$ | coinc | 36.11 | 25.63 | 35.79 | 26.93 | 128.52 | 9.01 |
| | DC | 0.09 | 0.19 | 0 | 0 | 0.28 | 0.28 |
| | idlers | $9.2\cdot10^4$ | $9.2\cdot10^4$ | $1.1\cdot10^5$ | $1.1\cdot10^5$ | $4\cdot10^5$ | $4\cdot10^5$ |
| **3 $\mu$s** | | $\|+\rangle\langle+\|$ | $\|-\rangle\langle-\|$ | $\|R\rangle\langle R\|$ | $\|L\rangle\langle L\|$ | $\|l\rangle\langle l\|$ | $\|e\rangle\langle e\|$ |
| $\hat{M}_i = \|+\rangle\langle+\|$ | coinc | 8.01 | 1.11 | 4.51 | 4.58 | 13.29 | 6.57 |
| | DC | 0.07 | 0.115 | 0.13 | 0.09 | 0.40 | 0.40 |
| | idlers | $1\cdot10^6$ | $1\cdot10^6$ | $8.6\cdot10^5$ | $8.6\cdot10^5$ | $3.7\cdot10^6$ | $3.7\cdot10^6$ |
| $\hat{M}_i = \|L\rangle\langle L\|$ | coinc | 5.20 | 3.72 | 8.89 | 0.95 | 12.02 | 6.96 |
| | DC | 0.08 | 0.117 | 0.1 | 0.12 | 0.41 | 0.41 |
| | idlers | $9.4\cdot10^5$ | $9.4\cdot10^5$ | $7.3\cdot10^5$ | $7.3\cdot10^5$ | $3.3\cdot10^6$ | $3.3\cdot10^6$ |
| $\hat{M}_i = \|e\rangle\langle e\|$ | coinc | 2.11 | 2.40 | 2.82 | 2.57 | 1.52 | 9.89 |
| | DC | 0.06 | 0.16 | 0.06 | 0.13 | 0.41 | 0.41 |
| | idlers | $3.1\cdot10^5$ | $3.1\cdot10^5$ | $3.2\cdot10^5$ | $3.2\cdot10^5$ | $1.3\cdot10^6$ | $1.3\cdot10^6$ |
| $\hat{M}_i = \|l\rangle\langle l\|$ | coinc | 6.6 | 4.38 | 5.64 | 5.58 | 21.79 | 1.14 |
| | DC | 0.08 | 0.13 | 0.09 | 0.12 | 0.42 | 0.42 |
| | idlers | $3.8\cdot10^5$ | $3.8\cdot10^5$ | $3.4\cdot10^5$ | $3.4\cdot10^5$ | $1.4\cdot10^6$ | $1.4\cdot10^6$ |
| **10 $\mu$s** | | $\|+\rangle\langle+\|$ | $\|-\rangle\langle-\|$ | $\|R\rangle\langle R\|$ | $\|L\rangle\langle L\|$ | $\|l\rangle\langle l\|$ | $\|e\rangle\langle e\|$ |
| $\hat{M}_i = \|+\rangle\langle+\|$ | coinc | 2.29 | 0.25 | 1.81 | 1.16 | 3.92 | 2.01 |
| | DC | 0.04 | 0.12 | 0.05 | 0.09 | 0.30 | 0.30 |
| | idlers | $7\cdot10^5$ | $7\cdot10^5$ | $5.8\cdot10^5$ | $5.8\cdot10^5$ | $2.6\cdot10^6$ | $2.6\cdot10^6$ |
| $\hat{M}_i = \|L\rangle\langle L\|$ | coinc | 1.23 | 1.45 | 2.46 | 0.46 | 3.47 | 2.00 |
| | DC | 0.05 | 0.09 | 0.06 | 0.07 | 0.27 | 0.27 |
| | idlers | $7\cdot10^5$ | $7\cdot10^5$ | $1\cdot10^6$ | $1\cdot10^6$ | $3.4\cdot10^6$ | $3.4\cdot10^6$ |
| $\hat{M}_i = \|e\rangle\langle e\|$ | coinc | 0.85 | 0.69 | 1.08 | 1.05 | 0.70 | 3.85 |
| | DC | 0.06 | 0.06 | 0.04 | 0.11 | 0.27 | 0.27 |
| | idlers | $3.2\cdot10^5$ | $3.2\cdot10^5$ | $2.9\cdot10^5$ | $2.9\cdot10^5$ | $1.2\cdot10^6$ | $1.2\cdot10^6$ |
| $\hat{M}_i = \|l\rangle\langle l\|$ | coinc | 1.72 | 1.3 | 1.70 | 1.63 | 6.62 | 0.64 |
| | DC | 0.06 | 0.08 | 0.09 | 0.09 | 0.32 | 0.32 |
| | idlers | $3.6\cdot10^5$ | $3.6\cdot10^5$ | $3.2\cdot10^5$ | $3.2\cdot10^5$ | $1.4\cdot10^6$ | $1.4\cdot10^6$ |

Table 1: Raw data of coincidence counts and dark counts (DC) per $10^4$ idler counts, measured in a 400 ns window.

| | **Raw** | $\widetilde{M}(\phi)$ | **uMZI** | **DC** | **280ns** |
|---|---|---|---|---|---|
| **Input** | 75.4(2.1) | 75.5(2.1) | 80.6(2.3) | 80.8(2.4) | 83.7(2.7) |
| **3 $\mu$s** | 79.2(1.8) | 79.6(1.8) | 84.8(1.9) | 85.9(2.0) | 87.3(2.0) |
| **10 $\mu$s** | 76.9(3.1) | 77.8(3.1) | 82.2(3.3) | 86.3(3.5) | 87.8(3.7) |

Table 2: Fidelities to the ideal case for the input state and for the two storage times. Each column represents a different analysis setting, which is applied additionally with the previous ones (e.g. the last column has all the previous corrections). Raw: raw data. $\widetilde{M}(\phi)$: data analysed with exact projective measurements. uMZI: data corrected for the imperfect analyser. DC: data corrected for dark counts. 280 ns: the coincidences are collected in a 280 ns window, instead of 400 ns.

estimation process we included an additional sampling of the distribution of phase settings for both interferometers, considering now the error on those values to be Gaussian.

A second correction that can be applied to the data is related to the interferometers used to analyse the entangled state of signal and idler. As mentioned in the main text, the signal interferometer is particularly unbalanced, due to the presence of fibre-to-fibre connectors and of the inherent loss of the 85 m fibre spool. Therefore, photons traveling through the long arm experience twice as much loss as they would through the short one. This will result in an imbalance between the projective measurements on $|e\rangle$ and $|l\rangle$ for the signal, and in a visibility of interference limited to about 95%. These imperfections reduce the final fidelity of the tomography, but since they are related to the analysis of the entanglement and not to the generation nor the storage, we believe it is fair to correct for them. Consequently, we corrected the coincidences measured in the right-most peaks of the histograms in Fig. 2 by renormalising them to the ratio between the transmission through the late and early arm (49%) of the signal interferometer. To account for the limited visibility instead, we note that it is possible to write:

$$m_j = \frac{N_j}{N_j + N_j'} = \frac{1+V_j}{2} \tag{2}$$

where $V_j = \left(N_j - N_j'\right) / \left(N_j + N_j'\right)$ is the visibility of the measurement for the j-th case. For the measurements on $\hat{M}_{\text{s}}(0) = |+/-\rangle\langle+/-|$ and $\hat{M}_{\text{s}}(\pi/2) = |R/L\rangle\langle R/L|$ this visibility includes the contribution of the signal interferometer, and it can then be factored out. For these cases we calculated the visibility $V_j$ from the measured coincidences, calculated a new visibility $V_j' = V_j/0.95$ and recalculated the new $m_j' = \frac{1+V_j'}{2}$. The values of fidelities obtained including these corrections are also reported in Tab. 2, and are slightly improved with respect to the previous ones. The idler interferometer has an identical design to the signal one, but the unbalance is less pronounced due to the low losses in fibre for telecom light.

Finally, we corrected the fidelities to account for the dark counts of our system. We measured the dark counts in a temporal window where the pump laser was off, and after the echo in case of AFC storage (the black shaded regions in Fig. 2). From these coincidences we estimated

| **In** | $\langle ee\vert$ | $\langle el\vert$ | $\langle le\vert$ | $\langle ll\vert$ |
|---|---|---|---|---|
| $\vert ee\rangle$ | 0.447 | -0.009 - i 0.035 | 0.005 + i 0.002 | 0.351 - i 0.056 |
| $\vert el\rangle$ | -0.009 + i 0.035 | 0.053 | 0.03 + i 0.001 | -0.004 - i 0.002 |
| $\vert le\rangle$ | 0.005 - i 0.002 | 0.03 - i 0.001 | 0.033 | 0.048 - i 0.037 |
| $\vert ll\rangle$ | 0.351 + i 0.056 | -0.004 + i 0.002 | 0.048 + i 0.037 | 0.468 |

| **3 $\mu s$** | $\langle ee\vert$ | $\langle el\vert$ | $\langle le\vert$ | $\langle ll\vert$ |
|---|---|---|---|---|
| $\vert ee\rangle$ | 0.464 | -0.004 - i 0.023 | -0.005 + i 0.016 | 0.382 + i 0.031 |
| $\vert el\rangle$ | -0.004 + i 0.023 | 0.03 | -0.004 - i 0.003 | 0.009 - i 0.005 |
| $\vert le\rangle$ | -0.005 - i 0.016 | -0.004 + i 0.003 | 0.017 | 0.045 - i 0.005 |
| $\vert ll\rangle$ | 0.382 - i 0.031 | 0.009 + i 0.005 | 0.045 + i 0.005 | 0.489 |

| **10 $\mu s$** | $\langle ee\vert$ | $\langle el\vert$ | $\langle le\vert$ | $\langle ll\vert$ |
|---|---|---|---|---|
| $\vert ee\rangle$ | 0.466 | 0.028 - i 0.008 | -0.014 - i 0.003 | 0.391 - i 0.088 |
| $\vert el\rangle$ | 0.028 + i 0.008 | 0.032 | 0.008 - i 0.016 | 0.019 - i 0.01 |
| $\vert le\rangle$ | -0.014 + i 0.003 | 0.008 + i 0.016 | 0.024 | 0.033 + i 0.003 |
| $\vert ll\rangle$ | 0.391 + i 0.088 | 0.019 + i 0.01 | 0.033 - i 0.003 | 0.477 |

Table 3: Density matrices for the three cases depicted in Fig. 3 of the main text, with full corrections applied.

the mean number of counts in a 400 ns window, and subtracted them from the measured coincidences. As can be noted from the last column of Tab. 2, this correction improved the case of 10 $\mu$s storage the most, due to its low count rate. Nevertheless, the final fidelity was similar to that of 3 $\mu$s storage, a sign of consistency between the two measurements. The density matrices for all three cases and with all the corrections are reported in Tab. 3.

These last values of fidelities are those reported in the main text. They were calculated considering windows of 400 ns, which contains 92% of the photon wavefunction. Higher values of fidelities can be obtained by considering smaller windows. Examples for a 280 ns window, whichs contains 78% of the photons, are reported in the last column of Tab. 2.

All of the corrections applied to the data account only for imperfections in the analysis of the entanglement, and therefore we believe them to be fair. A bigger limitation is actually given by the linewidth of the pump laser, but since this is related to the quality of the entanglement generation, we believe this factor could not be eliminated.

# References

[1] Seri, A. *et al.* Laser-written integrated platform for quantum storage of heralded single photons. *Optica* **5**, 934 (2018).

[2] Seri, A. *et al.* Quantum Storage of Frequency-Multiplexed Heralded Single Photons. *Physical Review Letters* **123**, 080502 (2019).

[3] Altepeter, J. B., James, D. F. & Kwiat, P. G. Qubit Quantum State Tomography. In *Quantum State Estimation*, 113–145 (2004). URL http://link.springer.com/10.1007/978-3-540-44481-7_4.
